# Supplementary material for: Random Function Descent
Source: arXiv:2305.01377 source file (2024-10-15)
Supplement: Supplementary file 1 [file appendix_random_regression.tex]

\section{Appendix: Random Regression}
\subsection{Proof of Theorem~\ref{thm: general regression decomposition}}

\begin{enumerate}
	\item \textbf{Expectation:}
	Using the independence of the measurement error \(\noise\) we get
	\begin{align*}
		&\mu_\Cost(\param) - \tfrac12\E\|\noise\|^2
		\\
		&= \E[\Cost(\param)] - \tfrac12\E\|\noise\|^2
		\\
		&= \E\Bigl[
			\tfrac12\Bigl\|\bigl(f_\param(X) -\mu_{\rf}(X)\bigr)
			- \bigl(\rf(X) - \mu_{\rf}(X)\bigr)\Bigr\|^2
		\Bigr]
		\\
		&= \begin{aligned}[t]
			&\tfrac12\E\|f_\param(X) -\mu_{\rf}(X)\|^2 
			\\
			&-\E\Bigl[
				\Bigl\langle
						f_\param(X) - \mu_{\rf}(X),
						\underbrace{\E[\rf(X)-\mu_{\rf}(X)\mid X]}_{=0}
				\Bigr\rangle
			\Bigr]
			\\
			&+ \tfrac12\E\Bigl[
				\underbrace{\E[\|\rf(X) - \mu_{\rf}(X)\|^2\mid X]}_{=\trace \C_{\rf}(X, X)}
			\Bigr]
		\end{aligned}
		\\
		&=\tfrac12\E\|f_\param(X) -\mu_{\rf}(X)\|^2 + \tfrac12\E[\trace\C_{\rf}(X,X)].
	\end{align*}

\item \textbf{Batch normalization}
	At first it seems like we do not have a constant expectation (which also
	means that \(\Cost\) can not be isotropic). But batch normalization
	ensures for each component \(j\)
	\[
		 \frac1n\sum_{i=1}^n f_\param(X_i)_j = 0,
		 \qquad
		 \frac1n\sum_{i=1}^n (f_\param(X_i))_j^2 = 1.
	\]
	For large datasets \(n\to \infty\), this essentially ensures standardization for every
	output dimension \(j\)
	\[
		 \E[f_\param(X)_j] = 0,
		 \qquad 
		 \E[(f_\param(X))_j^2] = 1,
	\]
	which finally ensures constant expectation
	\begin{align*}
		 &\E\|f_\param(X)-\mu_{\rf}\|^2
		 \\
		 &= \E\|f_\param(X)\|^2 - 2\langle \E[f_\param(X)], \mu_{\rf}\rangle + \|\mu_{\rf}\|^2
		 \\
		 &= \sum_{j=1}^\dims \E\Bigl[
			  (f_\param(X))_j^2
		 \Bigr] - \|\mu_{\rf}\|^2
		 \\
		 &= \dims - \|\mu_{\rf}\|^2 = \text{const.}
	\end{align*}

	\item \textbf{Decomposition:}

	So let us now consider the centered loss
	\begin{align*}
		 &\bar{\Cost}(\param)
		 \\
		 &= \Cost(\param) - \teal{\mu_\Cost(\param)}
		 \\
		 &= 
		 \begin{aligned}[t]
			  &\underbrace{
				\begin{aligned}[t]
					&\tfrac12\E\Bigl[ \|f_\param(X) - \mu_{\rf}(X)\|^2 \mid \rf \Bigr]
					\\
					&\qquad - \teal{\tfrac12\E\|f_\param(X) - \mu_{\rf}(X)\|^2}
				\end{aligned}
				}_{=0}
			  \\
			  &\underbrace{-
					\E\Bigl[\bigl\langle f_\param(X) - \mu_{\rf}(X), \rf(X) -\mu_{\rf}(X) \bigr\rangle \Bigm| \rf\Bigr]
			  }_{ =:\hat{\Cost}(\param)}
			  \\
			  &+ \underbrace{
				\begin{aligned}[t]
					&\Bigl(\tfrac12\E\Bigl[\|\rf(X)-\mu_{\rf}(X)\|^2\mid \rf\Bigr] 
					\\
					&\qquad - \teal{\tfrac12\E[\trace\C_{\rf}(X,X)]}\Bigr)
				\end{aligned}
				}_{=:Z}
		 \end{aligned}
	\end{align*}

	\item \textbf{Gaussian:}
	If \(\rf\) is Gaussian, then as a linear combination of centered Gaussian
	random variables \(\rf(x) - \mu_{\rf}(x)\),
	\[
		 \hat{\Cost}(\param)
		 = -\int \bigl\langle f_\param(x) - \mu_{\rf}(x), \rf(x) -\mu_{\rf}(x) \bigr\rangle \Pr_X(dx)
	\]
	is centered Gaussian, since the integral is a centered Gaussian random
	variable because limits of centered Gaussian random variables are
	centered Gaussian. 

	\item \textbf{Covariance:}
	What is left is the covariance function of \(\hat{\Cost}\):
	\begin{align*}
		 &\E[\hat{\Cost}(\param_1) \hat{\Cost}(\param_2)]
		 \\
		 &= \iint
		 \begin{aligned}[t]
			  \E\Bigl[
					&\bigl\langle f_{\param_1}(x) - \mu_{\rf}(x), \rf(x) -\mu_{\rf}(x) \bigr\rangle
					\\
					&\cdot\bigl\langle f_{\param_2}(y) - \mu_{\rf}(y), \rf(y) -\mu_{\rf}(y) \bigr\rangle
			  \Bigr]
			  \\
			  &\Pr_X(dx) \Pr_X(dy)
		 \end{aligned}
		 \\
		 &= \iint
		 \begin{aligned}[t]
			  &(f_{\param_1}(x)-\mu_{\rf}(x))^T
			  \\
			  &\underbrace{
					\E\Bigl[
					(\rf(x) -\mu_{\rf}(x))
					(\rf(y) -\mu_{\rf}(y))^T
			  \Bigr]
			  }_{=\C_{\rf}(x,y)}&&
			  \\
			  &\cdot (f_{\param_2}(y)-\mu_{\rf}(y))
			  \quad \Pr_X(dx) \Pr_X(dy)
		 \end{aligned}
	\end{align*}
	which finishes the proof. \qedhere
\end{enumerate}
