# Supplementary material for: Random Function Descent
Source: arXiv:2305.01377 source file (2024-10-15)
Supplement: Supplementary file 2 [file random_function_appendix.tex]

\section{Random functions}\label{sec: random function}

\begin{definition}[Random function]
	A family of random variables \((Z(x))_{x\in\real^\dims}\) is a 
	\emph{random function} over \(\real^\dims\).

\end{definition}
\begin{definition}[Strict stationarity]\label{def: strict stationarity}
	A random function \(Z\) is called \emph{(strictly) stationary} if it is
	invariant to shifts in distribution, i.e.
	\[
		(Z(x_1),\dots, Z(x_k)) \overset{d}= (Z(x_1 + \step),\dots, Z(x_k+\step))
		\quad\forall \step\in\real^\dims.
	\]
\end{definition}

\begin{definition}[Covariance function]\label{def: covariance function}
	The covariance function of a random function \(Z\) is defined as
	\begin{equation}
		\Cf(x,y):= \Cov(Z(x), Z(y)).
	\end{equation}
\end{definition}

\begin{definition}[Weak stationarity]
	A random function \(Z\) is called \emph{(weakly) stationary}, if for all
	\(x,y\in\real^\dims\)
	\[
		\Cf(x,y) = \Cf(x-y)
	\]
	and \(\E[Z(x)]=\mu\) for a fixed \(\mu\in\real^\dims\).
\end{definition}

\begin{remark}
	Strictly stationary implies weakly stationary. The definitions coincide for
	Gaussian random variables. Throughout this paper we use ``stationary''
	for ``weakly stationary''.
\end{remark}

\begin{definition}[Isotropy]
	A stationary random function \(Z\) is called \emph{isotropic} if the covariance
	is also rotation invariant, i.e.
	\[
		\Cf(x,y) = \Cf(x-y)= \sqC(\|x-y\|^2).
	\]
\end{definition}

\begin{definition}[Intrinsic stationarity]
	\label{def: variogram}
	A random function \(Z\), for which its increments
	\[
		Z_\step(x) := Z(x+\step)- Z(x)
	\]
	are stationary for every \(\step\), is called \emph{intrinsically stationary}
	if its mean is continuous.
	For any intrinsically stationary random function, the \emph{(centred) variogram} is
	defined as
	\[
		\variogram(\step)	= \tfrac12\Var(Z_\step(x)),
	\]
	which is independent of \(x\) due to stationarity of \(Z_\step\). For the
	uncentered variogram use uncentered second moments instead of the variance.
\end{definition}

\begin{lemma}[Intrinsically stationary mean]
	An intrinsically stationary random function \(Z\) has mean
	\[
		\E[Z(x)] = \underbrace{\E[Z(0)]}_{\mu_0} + \langle \mu_\grad, x\rangle
	\]
	for some \(\mu_\grad\in\real^\dims\). If \(Z\) is differentiable, we
	therefore have
	\[
		\E[\grad Z(x)] = \grad \E[Z(x)] = \mu_\grad.
	\]
\end{lemma}
\begin{proof}
	As \(Z_\step\) is stationary,
	\[
		\mu(\step):= \E[Z_\step(x)] = \E[Z(x+\step)-Z(x)]
	\]
	is well defined. We therefore have
	\[
		\E[Z(\step)] = \E[Z(0)] + \mu(\step),
	\]
	so if we can prove \(\mu\) is linear we are done. Additivity is easy 
	\[
		\mu(\step_1+\step_2)
		= \underbrace{\E[Z(x+\step_1+\step_2)-Z(x+\step_1)]}_{=\mu(\step_2)}
		+ \underbrace{\E[Z(x+\step_1)-Z(x)]}_{\mu(\step_1)}.
	\]
	For scalability we start with natural numbers
	\[
		\mu(m\step) = \sum_{k=1}^m \underbrace{\E[Z(x+k\step)-Z(x+(k-1)\step)]}_{\mu(\step)}
		= m\mu(\step).
	\]
	As this implies \(\mu(\step) = \mu(m \frac1m \step) = m \mu(\frac1m \step)\),
	we can generalize this to rational factors. To finish the proof we apply
	the continuity of the mean we required in the definition of intrinsic
	stationarity.
\end{proof}

\begin{lemma}[Covariance from Variogram]
	\label{lem: covariance from variogram}
	If \(Z\) is intrinsically stationary we have for \(Y_s := Z - Z(s)\)
	and
	\[
		\Cf_s(x,y) := \Cov(Y_s(x), Y_s(y)) = \Cov(Z_{x-s}(s), Z_{y-s}(s))
	\]
	an explicit representation using the variogram
	\begin{align*}
		\Cf_s(x,y)
		&= \variogram(x-s) + \variogram(y-s) - \variogram(x-y)\\
		\overset{\text{symm.}}&= \variogram(x-s) + \variogram(y-s) - \variogram(y-x)
	\end{align*}
\end{lemma}
\begin{remark}[Antisymmetry]\label{rem: grad variogram antisymmetric}
	We therefore have \(\variogram(x-y) = \variogram(y-x)\) or in other words
	the variogram is symmetric. So if it is differentiable, then
	\(\grad\variogram\) is antisymmetric with \(\grad\variogram(0)=0\).
\end{remark}
\begin{proof}[Proof (suggested to us by Martin Schlather in verbal communication)]
	Assume \(Z\) is centred without loss of generality, otherwise center \(Z\)
	resulting in \(\tilde{Z}\) and notice that \(\tilde{Y}_s\) is the centered
	version of \(Y_s\)
	\begin{align*}
		\Cf_s(x,y) 
		&= \E[(Z(x) - Z(s))(Z(y)-Z(s))]\\
		&= \E[(Z(x) - Z(y) + Z(y) - Z(s))(Z(y) - Z(x) + Z(x) - Z(s))]\\
		&=\begin{aligned}[t]
			-&\E[(Z(x) - Z(y))^2] &&+ \underbrace{\E[(Z(x)-Z(y))(Z(x)-Z(s))]}_{=:I}\\
			+&\Cf_s(y,x)	&&+ \underbrace{\E[(Z(y) - Z(s))(Z(y) - Z(x))]}_{=:II}
		\end{aligned}
	\end{align*}
	And we have
	\begin{align*}
		I&=\E[(Z(x)- Z(s) + Z(s) - Z(y))(Z(x) - Z(s))]\\
		&= 2\variogram(x-s) - \Cf_s(y,x)
	\end{align*}
	and similarly \(II = 2\variogram(y-s) - \Cf_s(y,x)\). Together this
	results in
	\[
		\Cf_s(x,y) = -2\variogram(x-y) + 2\variogram(x-s) - \Cf_s(y,x) + 2\variogram(y-s) - \cancel{\Cf_s(y,x)} + \cancel{\Cf_s(y,x)}.
	\]
	Reordering and symmetry of the covariance results in the claim.
\end{proof}

\subsection{Derivatives of random functions}

The takeaway from the following proposition should be that it is essentially
always possible to swap integration with differentiation. This result is
certainly not new, but proving it turned out to be easier than finding a
good reference, and this ensures subsequent statements are more self contained.

The continuity assumption is the strongest requirement. This
can be lifted if one were satisfied with equality in the sense of distributions.
This is because the product of any function with an infinitely differentiable
test function is certainly continuous, so we do not have to worry about
continuity. A proof for this general case is said to be found in
\citet{jonesTheoryGeneralisedFunctions1982}.

\begin{prop}[Swapping integration and differentiation]
	\label{prop: swap integration and differentiation}
	Let \(f: U\times \Omega \to \real\) be a measurable function for
	\(U\subseteq \real\) which satisfies
	\begin{enumerate}[noitemsep,topsep=0pt]
		\item \(f\) \(\mu\)-integrable over \(\omega\in\Omega\) at
		\(t_0\in U\),
		
		\item for \(\mu\)-almost all \(\omega\in\Omega\) we have: \(t\to
		f(t,\omega)\) is differentiable (or absolutely continuous) in \(t\).

		\item
		If \(\frac{\partial}{\partial t}f\) is further ``locally integrable
		in \(t_0\)'', i.e.  there exists \(a<b\in\real\), such that
		\(t_0\in[a,b]\subseteq U\) and
		\[
			\exists a<b \in \real:
			\quad
			t_0\in[a,b]\subseteq U,\quad
			\int_a^b \int_\Omega
			\left|\frac{d}{dt}f(t,\omega)\right| d\mu(\omega)dt<\infty,
		\]
		or \(\frac{\partial}{\partial t}f\ge 0\) in the neighborhood \([a,b]\).

		\item\label{it: continuity} In a similar local neighborhood \([a,b]\) of \(t_0\) assume that
		\[
			t\mapsto \int \frac{\partial}{\partial t}	f(t,\omega)d\mu(\omega)
		\]
		is continuous.
	\end{enumerate}
	then swapping derivative in \(t_0\) and integration over \(\omega\) is allowed
	\[
		\frac{\partial}{\partial t}\int f(t_0, \omega)d\mu(\omega)
		= \int \frac{\partial}{\partial t}f(t_0,\omega)d\mu(\omega).
	\]
\end{prop}

\begin{proof}
	Without loss of generality let \(t_0<b\). Then using Fubini and the fundamental
	theorem of calculus, we get
	\begin{align*}
		\frac{\partial}{\partial t}\int f(t_0,\omega)d\mu(\omega)
		\overset{\text{linear}}&= \lim_{\epsilon\to 0}\int
		\frac{f(t_0+\epsilon,\omega) - f(t_0,\omega)}{\epsilon}d\mu(\omega)\\
		\overset{\text{FTC II}}&= \lim_{\epsilon\to 0}\int
		\frac1\epsilon \int_{t_0}^{t_0+\epsilon}\frac{\partial}{\partial t} f(t,\omega) dt d\mu(\omega)\\
		\overset{\text{Fubini}}&=
		\lim_{\epsilon\to 0}\frac1\epsilon \int_{t_0}^{t_0+\epsilon}
		\int \frac{\partial}{\partial t}f(t,\omega) d\mu(\omega)dt \\
		\overset{\text{def.}}&=
		\frac{d}{dy} \int_{t_0}^{y}
		\int \frac{\partial}{\partial t}f(t,\omega) d\mu(\omega)dt\Biggr|_{y=t_0}\\
		\overset{\text{FTC I}}&=
		\int \frac{\partial}{\partial t}f(t_0,\omega) d\mu(\omega).
	\end{align*}
	For the last equality we needed the continuity (requirement \ref{it:
	continuity}.) to apply FTC I.  The integrability condition (3.) is needed for
	Fubini (so it can be replaced with
	a positivity condition).
\end{proof}

The requirements of the following lemma are vague on purpose to better convey
its spirit. This lemma is not new either, but the formal difficulties tend to
obscure this wonderful insight behind complicated requirements.
A formal treatment can be found in \citet{adlerRandomFieldsGeometry2007}
and the sharp edges of the requirements are discussed in the proof(sketch).

\begin{lemma}[Covariance and derivative]
	\label{lem: covariance of derivative}
	Let \(\Cost\) be a random function. Then we have
	\begin{align*}
		\Cov(\partial_i\Cost(x), \Cost(y)) &= \partial_{x_i} \Cf(x,y)\\
		\Cov(\partial_i\Cost(x), \partial_j \Cost(y)) &= \partial_{x_i y_j} \Cf(x,y),
	\end{align*}
	essentially if \(\partial_i\Cost\) is well defined.
\end{lemma}
\begin{proof}
	We assume \(\E[\Cost(x)] =0\) without loss of generality. Then covariance
	is just a product of expectations. So we get
	\[
		\Cov(\partial_i \Cost(x), \Cost(y))
		= \E[ \partial_{x_i} \Cost(x) \Cost(y)]
		= \partial_{x_i} \E[\Cost(x) \Cost(y)]
		\overset{\text{def.}}= \partial_{x_i}\Cf(x,y)
	\]
	because swapping integration and differentiation is essentially always possible 
	(Prop.~\ref{prop: swap integration and differentiation}).

	It is a much more delicate question, whether the derivative \emph{exists}. To
	ensure this is the case, slightly stronger requirements on the covariance
	function are usually assumed \citep{adlerRandomFieldsGeometry2007}, which
	ensure the existence \emph{and continuity} of \(\partial_i \Cost\) and at that
	point we do not have to worry about continuity for the application of
	Prop.~\ref{prop: swap integration and differentiation} anymore.
	If one were able to define \(\partial_i \Cost\) as a random
	generalized function (distribution), one could still swap integration with
	differentiation since equality then only matters in the sense of
	distributions.
\end{proof}
\begin{remark}\label{rem: antisymmetry}
	For stationary random functions \(\Cf(x,y)=\Cf(x-y)\), the covariance
	function \(\Cf\) is symmetric, i.e. \(\Cf(h)=\Cf(-h)\)
	and therefore the derivative antisymmetric, i.e.
	\(\partial_i\Cf(-h)=-\partial_i\Cf(h)\). In particular
	\begin{equation*}
		\Cov(\grad\Cost(x), \Cost(x)) = \grad \Cf(0)=0.
	\end{equation*}
\end{remark}
\begin{corollary}[Gaussian Case]
	If \(\Cost\) is a stationary gaussian random function, \(\Cost(x)\) and
	\(\grad\Cost(x)\) are independent multivariate gaussian for every \(x\).
\end{corollary}

\begin{lemma}[Variogram and Derivative]\label{lem: variogram and derivative}
	Assuming \(Z\) is an intrinsically stationary, differentiable random function,
	we have
	\begin{enumerate}
		\item \(
			\Cov(Z(x+\step)-Z(x), \grad Z(x)) = \grad\variogram(\step)
		\)
		\item \(\Cov(\grad Z(x), \grad Z(y)) = \grad^2\variogram(x-y)\)
		(this implies \(\grad Z\) is stationary)
		\item \(\Cov(Z(x+\step)-Z(x),\hessian Z(x))
		= \hessian\variogram(0) - \hessian\variogram(\step)\)
	\end{enumerate}
\end{lemma}
\begin{proof}
	\begin{enumerate}[wide]
	\item We have
	\begin{equation*}
		\partial_i Z(x) = \lim_{h\to 0}\frac{Z(x + he_i) - Z(s) -(Z(x)-Z(s))}{h}
		= \partial_i Y_s(x) \quad \forall x,s
	\end{equation*}
	and therefore
	\begin{equation*}
		\Cov(\partial_i Z(x), Z(x+\step)-Z(x))
		\overset{\text{Lem~\ref{lem: covariance of derivative}}}=
		\partial_{x_i}\Cf_x(x, x+\step)
		= \underbrace{\partial_i\variogram(0)}_{
			=0 \mathrlap{\text{ (Remark~\ref{rem: grad variogram antisymmetric})}}
		}
		- \partial_i\variogram(-\step),
	\end{equation*}
	because the variogram is symmetric and the derivative therefore antisymmetric.

	\item Here we use \(\partial_i Z(x) = \partial_i Y_s(x)\) again
	\begin{align*}
		\Cov(\partial_i Z(x), \partial_j Z(y))
		&= \Cov(\partial_i Y_s(x), \partial_j Y_s(y))\\
		\overset{\text{Lem~\ref{lem: covariance of derivative}}}&=
		\partial_{y_j x_i} \Cf_s(x,y)\\
		\overset{\text{Lem~\ref{lem: covariance from variogram}}}&=
		\partial_{y_j x_i} [\variogram(x-s) + \variogram(y-s) - \variogram(x-y)]\\
		&= \partial_{y_j} [\partial_i\variogram(x-s) - \partial_i\variogram(x-y)]\\
		&= \partial_{ij}\variogram(x-y).
	\end{align*}

	\item Using the previous results about gradients, we get
	\begin{align*}
		&\tfrac1h\Cov(\grad Z(x+h e_i) -\grad Z(x), Z_\step(x))\\
		&= \tfrac1h\begin{aligned}[t]
			\bigg[&\Cov(\grad Z(x+h e_i), Z(x+\step) - Z(x+h e_i))\\
			&+ \Cov(\grad Z(x+h e_i), Z(x+h e_i) - Z(x))\\
			&- \Cov(\grad Z(x), Z_x(\step))\bigg]
		\end{aligned}
		\\
		&= \tfrac1h[\grad\variogram(\step - h e_i) - \grad\variogram(-h e_i) - \grad(\step)]\\
		&= \tfrac1h[(\grad\variogram(h e_i) - \grad\variogram(0)) -(\grad\variogram(\step) - \grad\variogram(\step -h e_i))]\\
		&\to \partial_i\grad\variogram(0) - \partial_i\grad\variogram(\step)
	\end{align*}
	where we have used antisymmetry of \(\grad\variogram\) for the last equation.
	\qedhere

	\end{enumerate}

	\begin{lemma}[Derivatives of Rotation Invariant Variograms]
	\label{lem: derivatives of rotation invariant variograms}
		For a rotation invariant variogram \(\variogram(\step) = \phi(\|\step\|^2)\),
		we have
		\begin{enumerate}
			\item
			\(\grad \variogram(\step) = 2\phi'(\|\step\|^2) \step\)
			\item
			\(\grad^2 \variogram(\step)
			= 4 \phi''(\|\step\|^2) \step \step^T + 2\phi'(\|\step\|^2)\identity\)
			\item
			\(\partial_{kij}\variogram(\step) = 8\phi'''(\|\step\|^2)\step_k\step_i\step_j
			+ 4\phi''(\|\step\|^2)[\delta_{ki}\step_j + \delta_{kj}\step_i + \delta_{ij}\step_k]
			\)
			\item
			\(\partial_{lkij}\variogram(0)
			= 4\phi''(0)[\delta_{ki}\delta_{jl} + \delta_{kj}\delta_{il} + \delta_{ij}\delta_{kl}]\)
		\end{enumerate}
	\end{lemma}
	\begin{proof}
		Product and chain rule.
	\end{proof}

\end{proof}
