# Supplementary material for: Random Function Descent
Source: arXiv:2305.01377 source file (2024-10-15)
Supplement: Supplementary file 3 [file rfd_appendix.tex]

\section{RFD details}\label{sec: rfd appendix}

We will present the most general version of the results here. This
means:
\begin{enumerate}
	\item
	We avoid the Gaussian assumption using the \(\BLUE\) we defined in
	Section~\ref{sec: BlUE} with Lemma~\ref{lem: blue is cond. expectation}
	in mind for the Gaussian case.

	\item 
	We make the generalization over isotropy, using
	\[
		\langle x, y\rangle_A := \langle x, Ay\rangle
	\]
	for some symmetric, positive definite \(A\) which also induces \(\|x\|_A\).
	Isotropy is then replaced by \(\Cf(x,y) = \sqC(\|x\|_A^2)\).

	\item We consider sample losses
	\[
		\loss(\param, Z) = \Cost(\param) + \epsilon_0
		\qquad
		\nabla\loss(\param, \tilde{Z}) = \nabla\Cost(\param) + \epsilon_1
	\]
	where the errors \(\epsilon_0, \epsilon_1\) have zero expectation, finite
	variance, are uncorrelated and also not correlated with \(\Cost\).
	\(\epsilon_0\) and \(\epsilon_1\) being uncorrelated likely requires
	\(\tilde{Z}\) is a different data sample than \(Z\) although in practice this
	will likely be ignored.
\end{enumerate}

\subsection{Stationarity}

Under stationarity we have by Remark~\ref{rem: antisymmetry}
\[
	\Cov(\Cost(\param), \grad\Cost(\param))=0.
\]
So we can easily ``condition'' on both \(\Cost(\param)\) and
\(\grad\Cost(\param)\). The same translates to the sample losses, since
\(\epsilon_i\) are uncorrelated.

\begin{lemma}\label{lem: blue centered, stationary}
	Assume \(\Cost\) is a \textbf{stationary} and \textbf{differentiable} random
	function with covariance function \(\Cf\) and mean \(\mu=\E[\Cost(\param)]\).
	Using the notation \(\bar{\Cost}:=\Cost -\mu\) and
	\(\bar{\loss} := \loss - \mu\), we have
	\begin{align*}
		&\BLUE[
			\bar{\Cost}(\param + \step)
			\mid \loss(\param, Z), \grad\loss(\param, \tilde{Z})
		]\\
		&= \frac{\Cf(\step)}{\Cf(0)+\E[\epsilon_0^2]} \bar{\loss}(\param, Z)
		- \grad\Cf(\step)^T (-\grad^2\Cf(0) + \E[\epsilon_1\epsilon_1^T])^{-1} \grad\loss(\param, \tilde{Z})
	\\
	\intertext{
		if \(\Cost\) is additionally \textbf{isotropic}, i.e.
		\(\Cf(\step)=\sqC(\|\step\|_A^2)\) and \(\E[\epsilon_1\epsilon_1^T] =
		\sigma^2A\), this reduces to
	}
		&= \frac{\sqC(\|\step\|_A^2)}{\sqC(0)+ \E[\epsilon_0^2]}
		\bar{\loss}(\param, Z)
		- \frac{\sqC'(\|\step\|_A^2)}{\sigma^2 - \sqC'(0)}
		\langle \step, \grad\loss(\param, \tilde{Z})\rangle.
	\end{align*}
\end{lemma}
\begin{proof}
	By working with \(\bar{\Cost}\) (and \(\bar{\loss}\)) instead of \(\Cost\)
	(and \(\loss\)), we can assume without loss of generality that \(\Cost\) (and
	\(\loss\)) is centered. So we know that any  element
	\(\hat{\Cost}(\param + \step)\) from \(\LUE\) has the form
	\begin{equation*}
		\hat{\Cost}(\param + \step)
		= a\loss(\param, Z) + \langle b, \grad\loss(\param, \tilde{Z})\rangle
	\end{equation*}
	for \(a\in\real\), \(b\in \real^\dims\). So we want to minimize 
	\begin{align*}
		g(a,b)
		&=\E[\|\Cost(\param +\step) - \hat{\Cost}(\param + \step)\|^2]\\
		&= \begin{aligned}[t]
			&\E[\Cost(\param +\step)^2]\\
			&- 2a\underbrace{
				\E[\Cost(\param + \step)\loss(\param, Z)]
			}_{
				=\E[\Cost(\param + \step)\Cost(\param)]
			} + a^2
			\underbrace{
				\E[\loss(\param, Z)^2]
			}_{
				=\E[\Cost(\param)^2] + \E[\epsilon_0^2]
			}\\
			&- 2\langle b, \underbrace{
				\E[\Cost(\param + \step)\grad\loss(\param, \tilde{Z})]
			}_{
				= \E[\Cost(\param + \step)\grad\Cost(\param)]
			}\rangle
			+ \langle b, \underbrace{
				\E[\grad\loss(\param, \tilde{Z})\grad\loss(\param, \tilde{Z})^T]
			}_{
				= \E[\grad\Cost(\param)\grad\Cost(\param)^T] + \E[\epsilon_1 \epsilon_1^T]
			} b\rangle\\
			&- 2a\langle b, \underbrace{\E[\loss(\param, Z)\grad\loss(\param, \tilde{Z})]}_{
				=0\mathrlap{\text{ (Remark~\ref{rem: antisymmetry})}}
			}\rangle
		\end{aligned}\\
		&=\Cf(0) - 2a\Cf(\step) + a^2 (\Cf(0) + \E[\epsilon_0^2])
		- 2\langle b, \underbrace{\grad\Cf(-\step)}_{\overset{\ref{rem: antisymmetry}}=-\grad\Cf(\step)}\rangle
		+ \langle b, (-\grad^2\Cf(0) + \E[\epsilon_1\epsilon_1^T]) b\rangle
	\end{align*}
	with respect to \(a\) and \(b\), where we have used Lemma~\ref{lem:
	covariance of derivative} and stationarity for the last line. Fortunately
	there are no interactions between \(a\) and \(b\), as \(\Cost(\param)\) is
	uncorrelated from \(\grad\Cost(\param)\). First order conditions result in
	\begin{equation*}
		a= \frac{\Cf(\step)}{\Cf(0)+\E[\epsilon_0^2]}
		\quad \text{and} \quad
		b = -(-\grad^2 \Cf(0) + \E[\epsilon_1\epsilon_1^T])^{-1}\grad \Cf(\step).
	\end{equation*}
	These are minima, since \(-\grad^2\Cf(0)\) is positive definite, because of
	\begin{align*}
		\langle b, -\grad^2\Cf(0) b\rangle = \E[\langle b, \grad\Cost(\param)\rangle^2] \ge 0.
	\end{align*}
	Now we just need to address the \(\Cf(\step) = \sqC(\|\step\|_A^2)\) case. We have
	\begin{align*}
		\grad \Cf(\step) &= 2\sqC'(\|\step\|_A^2) A\step\\
		\grad^2 \Cf(\step)
		&= 4 \sqC''(\|\step\|_A^2) A\step \step^TA
		+ 2\sqC'(\|\step\|_A^2)A
	\end{align*}
	and therefore \(\grad^2\Cf(0) = 2\sqC'(0)A\). Plugging these results
	into the general formula together with \(\E[\epsilon_1\epsilon_1^T] =
	\sigma^2 A\) yields the claim
	\[
		\BLUE[\bar{\Cost}(\param + \step)\mid \Cost(\param), \grad\Cost(\param)]
		= \frac{\sqC(\|\step\|_A^2)}{\sqC(0)+\E[\epsilon_0^2]} \bar{\Cost}(\param)
		- \frac{\sqC'(\|\step\|_A^2)}{\sigma^2 - \sqC'(0)} \underbrace{(A\step)^T A^{-1}}_{=\step^T} \grad\Cost(\param).
		\qedhere
	\]
\end{proof}

\subsection{Intrinsic stationarity}

Intrinsic stationarity forces us to consider loss differences and stops us
from being able to condition on the loss itself. But we can still condition
on the gradient alone, as the gradient is a loss difference.

\begin{lemma}\label{lem: blue centered, intrinsically stationary}
	If \(\Cost\) is a \textbf{intrinsically stationary, differentiable}
	random function, with variogram \(\variogram\) and mean \(\E[\Cost(\param)] =
	\mu_0 + \langle \mu_\grad, \param\rangle\), then
	\begin{align*}
		&\BLUE[
			\underbrace{\Cost(\param+\step) - \Cost(\param)}_{=:\Cost_\param(\step)}
			\mid \grad\loss(\param, \tilde{Z})
		]\\
		&=  \langle \mu_\grad,\step\rangle + \grad\variogram(\step)^T(\grad^2\variogram(0)+\E[\epsilon_1\epsilon_1^T])^{-1}
		(\grad\loss(\param, \tilde{Z})-\mu_\grad)\\
		\intertext{
			if the variogram is \textbf{rotation invariant}, i.e.
			\(\variogram(\step)=\phi(\|\step^2\|_A)\), this simplifies to
		}
		&= \langle \mu_\grad,\step\rangle + \frac{\phi'(\|\step\|_A^2)}{\phi'(0)}
		\langle \step, \grad\loss(\param,\tilde{Z})-\mu_\grad\rangle
	\end{align*}
\end{lemma}
\begin{proof}
	Virtually identical to the stationary case, but using Lemma~\ref{lem: variogram
	and derivative} and Lemma~\ref{lem: derivatives of rotation invariant variograms}.
\end{proof}

\begin{remark}\label{rem: replace variogram with covariance}
	If \(\Cost\) is stationary we have \(\variogram(\step) = \Cf(0) - \Cf(\step)\).
	Therefore \(\grad\variogram = - \grad\Cf\) and \(\grad^2\variogram =
	-\grad^2\Cf\) which means we can replace the variogram
	with the covariance in this case.

	In the stationary case we also have \(\mu_\grad = 0\) and it does not matter
	whether one tries to estimate the loss difference \(\Cost_\param(\step)\) or
	\(\bar{\Cost}(\param+\step)\). That is because we have
	\[
		\BLUE[\Cost_\param(\step)\mid\grad\Cost(\param)]
		= \BLUE[\bar{\Cost}(\param+\step)\mid\grad\Cost(\param)]
		-\underbrace{\BLUE[\bar{\Cost}(\param)\mid\grad\Cost(\param)]}_{=0},
	\]
   as \(\Cost(\param)\) and \(\grad\Cost(\param)\) are uncorrelated (or
   independent in the gaussian case). So we get
	\begin{align*}
		\BLUE[\bar{\Cost}(\param + \step)\mid \grad\Cost(\param)]
		&= [\grad^2\Cf(0)]^{-1}\langle\grad\Cf(\step), \grad\Cost(\param)\rangle\\
		&= \frac{\sqC'(\|\step\|^2)}{\sqC'(0)}\langle \step, \grad\Cost(\param)\rangle.
	\end{align*}
	Notice that in the case \(\Cost(\param)=\mu\) or \(\bar{\Cost}(\param)=0\)
	this result coincides with the stationary case. So if we minimize the
	sophisticated estimator utilizing \(\Cost(\param)\)
	\[
		\BLUE[\Cost(\param+\step)\mid \Cost(\param), \grad\Cost(\param)],
	\]
	we can get the minimization of the
	simpler estimator
	\(
		\BLUE[\Cost(\param+\step)\mid \grad\Cost(\param)]
	\)
	for free by plugging in
	\(\bar{\Cost}(\param)=0\).
\end{remark}

\subsection{Random function descent}\label{subsec: rfd}

\begin{lemma}\label{lem: rotation invariant implies GD}
	Functions of the form
	\begin{equation*}
		B(\step)
		= g_0(\|\step\|_A^2) + g_1(\|\step\|_A^2)\langle \step, \grad\loss(\param, \tilde{Z})\rangle
	\end{equation*}
	are minimized by a gradient step (modified by \(A^{-1}\)), i.e.
	\[
		-\hat{\stepsize}\frac{A^{-1}\grad\loss(\param, \tilde{Z})}{\|A^{-1}\grad\loss(\param,\tilde{Z})\|_A}
		= \argmin_{\step}B(\step)
	\]
	with optimal step size
	\[
		\hat{\stepsize} \begin{aligned}[t]
			&=\argmin_{\stepsize} B\left(-\stepsize \tfrac{A^{-1}\grad\loss(\param, \tilde{Z})}{\|A^{-1}\grad\loss(\param, \tilde{Z})\|_A}\right)\\
			&= \argmin_{\stepsize} g_0(\stepsize^2) -  g_1(\stepsize^2)\stepsize\|A^{-1}\grad\loss(\param, \tilde{Z})\|_{A}
		\end{aligned}
	\]
\end{lemma}

\begin{proof}
	Essentially all the occurrences of \(\step\) in \(B\) are \(\|\cdot\|_A\)
	rotation invariant, so only the step size matters. The only place where that
	is not the case is the scalar product with the gradient. Therefore it
	determines the direction. We prove this by splitting the minimization problem
	\[
		\min_{\step} B(\step)
		= \min_{\stepsize\ge 0}\min_{\step:\|\step\|_A=\stepsize} B(\step)
		= \min_{\stepsize\ge 0}\min_{\step:\|\step\|_A=\stepsize}
		g_0(\stepsize^2)	
		+ g_1(\stepsize^2) \langle \step, \grad\loss(\param, \tilde{Z})\rangle.
	\]
	First we consider the inner optimization problem, depending on the
	sign of \(g_1(\stepsize^2)\), we either want to maximize or minimize
	\[
		\mathop{\text{opt}}_{\step: \|\step\|_A=\stepsize} \langle \step, \nabla\loss(\param, \tilde{Z})\rangle
		= \mathop{\text{opt}}_{\step: \|\step\|_A=\stepsize} \langle \step, A^{-1}\nabla\loss(\param, \tilde{Z})\rangle_A
	\]
	due to Cauchy-Schwarz we have
	\[
		-\underbrace{\|\step\|_A}_{=\stepsize} \|A^{-1}\nabla\loss(\param, \tilde{Z})\|_A
		\le \langle \step, A^{-1}\nabla\loss(\param, \tilde{Z})\rangle_A
		\le \underbrace{\|\step\|_A}_{=\stepsize} \|A^{-1}\nabla\loss(\param, \tilde{Z})\|_A
	\]
	where the inequalities are equalities for \(\step=\pm\stepsize
	\frac{A^{-1}\nabla\loss(\param, \tilde{Z})}{\|A^{-1}\nabla\loss(\param, \tilde{Z})\|_A}\).
	Since we minimized over positive \(\stepsize\) before, we can drop the \(\pm\) by
	allowing \(\stepsize<0\) to obtain
	\begin{align*}
		B(\step)
		&= \min_{\stepsize} g_0(\stepsize^2)	
			- g_1(\stepsize^2)\stepsize \|A^{-1}\grad\loss(\param, \tilde{Z})\|_A.
		\qedhere
	\end{align*}
\end{proof}

\begin{theorem}[Random Function Descent]\label{thm: rfd}
	(\(A\)-Distorted) stochastic gradient descent, i.e. 
	\begin{equation*}
		\step(\stepsize) 
		= - \frac{\stepsize}{\|A^{-1}\grad\loss(\param, \tilde{Z})\|_A} A^{-1}\grad\loss(\param, \tilde{Z})
		= - \tilde{\stepsize} A^{-1}\grad\loss(\param,\tilde{Z})
	\end{equation*}
	minimizes the 1-step 1-order \(\BLUE\) of \(A\)-rotation invariant random
	function \(\Cost\) in the following sense
	\begin{enumerate}
		\item for an \textbf{isotropic} random function \(\Cost\) with
		\(\Cf(\step)=C(\|\step\|_A^2)\) and
		\(\E[\epsilon_1\epsilon_1^T]=\sigma^2A\), we have
		\begin{align*}
			\step(\hat{\stepsize})
			&= \argmin_{\step}
			\BLUE[\Cost(\param + \step)\mid \loss(\param, Z), \grad\loss(\param, \tilde{Z})]\\
			\hat{\stepsize}
			&= \argmin_{\stepsize}\frac{\sqC(\stepsize^2)}{\sqC(0) + \E[\sigma_0^2]}
				\frac{\loss(\param,Z)-\mu}{\|A^{-1}\grad\loss(\param, \tilde{Z})\|_A}
			+  \stepsize\frac{\sqC'(\stepsize^2)}{\sigma^2 - \sqC'(0)}\\
			&= \argmin_{\stepsize}\frac{\sqC(\stepsize^2)}{\sqC(0)}
			\underbrace{
				\tfrac{\sqC(0)}{\sqC(0) + \E[\sigma_0^2]}
				\tfrac{\sigma^2 - \sqC'(0)}{-\sqC'(0)}
				\frac{\loss(\param,Z)-\mu}{\|A^{-1}\grad\loss(\param, \tilde{Z})\|_A}
			}_{=:\Theta}
			-  \stepsize\frac{\sqC'(\stepsize^2)}{\sqC'(0)}
		\end{align*}

		\item for a \textbf{intrinsically stationary, differentiable}
		random function \(\Cost\) with \textbf{centered increments} (\(\mu_\nabla = 0\)) and
		\textbf{rotation invariant} variogram \(\variogram(\step) =
		\phi(\|\step\|_A^2)\) and
		\(\E[\epsilon_1\epsilon_1^T]=\sigma^2A\), we have
		\begin{align*}
			\step(\hat{\stepsize})
			&= \argmin_{\step}
			\BLUE[\Cost(\param + \step) - \Cost(\param)\mid \grad\loss(\param,\tilde{Z})]\\
			\hat{\stepsize}
			&= \argmax_{\stepsize} \stepsize\frac{\phi'(\stepsize^2)}{\phi'(0) + \sigma^2}
		\end{align*}
	\end{enumerate}
\end{theorem}

\begin{proof}
	We simply apply Lemma~\ref{lem: rotation invariant implies GD}	to the results
	from Lemma~\ref{lem: blue centered, intrinsically stationary} and \ref{lem:
	blue centered, stationary} and note that the minimizer does not change if
	we divide the minimization problem by \(\|A^{-1}\grad\loss(\param,\tilde{Z})\|_A\).
\end{proof}

\subsection{Convergence considerations proofs}

\begin{lemma}[Convergence to stationary point of RFD]
	\label{lem-appdx: convergence to stationary point}
	If
	\(\stepsize^*(\Theta) \to 0\) implies \(\Theta\to -\infty\)
	and the parameters chosen by full gradient RFD converge \(\param_k \to
	\bar{\param}\) for \(k\to \infty\), then
	\[
		\|\nabla\Cost(\param_k)\| \to \|\nabla\Cost(\bar{\param})\| = 0.
	\]
	I.e. \(\bar{\param}\) is a stationary point.
\end{lemma}
\begin{proof}
	It is immediately clear that the step-sizes converge
	\[
		\stepsize_k^* = \|\param_{k+1} - \param_k\| \to 0.
	\]
	This implies by assumption 
	\[
		\Theta_k = \frac{\Cost(\param_k) - \mu}{\|\nabla \Cost(\param_k)\|} \to -\infty.
	\]
	But then we necessarily have
	\(\|\nabla\Cost(\param_k)\| \to 0 \)
	as \(\Cost(\param_k)\) is bounded (because \(\param_k \to \bar{\param}\) and \(\Cost\) is
	continuous). By continuity of \(\nabla\Cost\) we also have
	\(\|\nabla\Cost(\bar{\param})\|=0\).
\end{proof}

\subsubsection{The step size of RFD close to a critical point}
\label{subsec: step size close to critical point}

We want to analyze the behavior of
\[
	\frac{\stepsize^*}{\|\nabla\Cost(\param)\|}
\]
close to a critical point \(\param_*\) where \(\|\nabla\Cost(\param)\|=0\).
For the squared exponential model, the step size is given by
\[
	\stepsize^* = \Theta/2 + \sqrt{(\Theta/2)^2 + \scale^2}
	= \frac{-\Delta}{2\|\nabla\Cost\|} + \sqrt{\frac{\Delta^2}{4\|\nabla\Cost\|^2} + \scale^2}
\]
for \(\Delta := \mu - \Cost\). Therefore
\[
	\frac{\stepsize^*}{\|\nabla\Cost\|}
	= \frac{\sqrt{\frac{\Delta^2}4 + \scale^2 \|\nabla\Cost\|^2} - \frac{\Delta}2}{\|\nabla\Cost\|^2}.
\]
For
\[
	f(x) = \frac{\sqrt{c^2 + \scale^2 x} - c}{x}
\]
we have by L'Hôpital
\[
	\lim_{x\to 0} f(x)
	= \lim_{x\to 0}\frac{\tfrac12 (c^2 + \scale^2x)^{-1/2} \scale^2}{1} = \frac{\scale^2}{2c}.
\]
We therefore have in the vicinity of \(\param_*\) where \(\|\nabla\Cost(\param)\|\to \|\nabla\Cost(\param_*)\|=0\)
\[
	\lim_{\param \to \param_*}\frac{\stepsize^*}{\|\nabla\Cost(\param)\|}
	= \frac{\scale^2}{\Delta} = \frac{\scale^2}{\mu-\Cost(\param)}.
\]
