# Supplementary material for: Random Function Descent
Source: arXiv:2305.01377 source file (2024-10-15)
Supplement: Supplementary file 4 [file appendix_further_discussion.tex]

\section{Extended Case Study}
